# Supplementary material for: Co-design of Embodied Neural Intelligence via Constrained Evolution
Source: arXiv:2205.10688 source file (2022-05-21)
Supplement: Supplementary file 1 [file 09-appendix.tex]

\section{Appendix}

\setcounter{table}{0}

\begin{table*}[!htb]
\scriptsize
\begin{tabular}{lllllllllll}
\toprule
\multicolumn{11}{c}{\textbf{Baseline}}                                                                                                                                  \\
\midrule
& \textbf{Length}  & \textbf{Radius}      & \textbf{Density}     & \textbf{Initial Pos}  & \textbf{Initial Dir} $x$ & \textbf{Initial Dir} $y$ & \textbf{Initial Dir} $z$ & \textbf{Stiffness}    & \textbf{Damping}     & \textbf{Max Effort}              \\
\midrule
\textbf{avg}   & 0.66 & 0.07  & 5.00  & 0.73 & 0.00   & -0.27  & -0.30  & 50.00 & 15.00          & 20.00  \\
body 0  & 0.30 & 0.10  & 5.00  & 0.00 & 0.00   & -1.00  & 0.00   & 50.00 & 15.00          & 20.00  \\
body 1  & 0.40 & 0.06  & 5.00  & 0.20 & 0.71   & 0.71   & 0.00   & 50.00 & 15.00          & 20.00  \\
body 2  & 0.40 & 0.06  & 5.00  & 0.20 & -0.71  & 0.71   & 0.00   & 50.00 & 15.00          & 20.00  \\
body 3  & 1.20 & 0.06  & 5.00  & 1.00 & 0.41   & 0.41   & -0.82  & 50.00 & 15.00          & 20.00  \\
body 4  & 1.20 & 0.06  & 5.00  & 1.00 & -0.41  & 0.41   & -0.82  & 50.00 & 15.00          & 20.00  \\
body 5  & 0.30 & 0.10  & 5.00  & 1.00 & 0.00   & -1.00  & 0.00   & 50.00 & 15.00          & 20.00  \\
body 6  & 0.30 & 0.10  & 5.00  & 1.00 & 0.00   & -1.00  & 0.00   & 50.00 & 15.00          & 20.00  \\
body 7  & 0.40 & 0.06  & 5.00  & 0.80 & 0.71   & -0.71  & 0.00   & 50.00 & 15.00          & 20.00  \\
body 8  & 0.40 & 0.06  & 5.00  & 0.80 & -0.71  & -0.71  & 0.00   & 50.00 & 15.00          & 20.00  \\
body 9  & 1.20 & 0.06  & 5.00  & 1.00 & 0.41   & -0.41  & -0.82  & 50.00 & 15.00          & 20.00  \\
body 10 & 1.20 & 0.06  & 5.00  & 1.00 & -0.41  & -0.41  & -0.82  & 50.00 & 15.00          & 20.00  \\
\midrule
\multicolumn{11}{c}{\textbf{Evolved} (fixed torso)}                                                                                                                          \\
\midrule
\textbf{avg}    & 0.70 & 0.07  & 4.81  & 0.73 & 0.00   & -0.21  & -0.26  & 49.69 & 15.55          & 22.56  \\
body 0  & 0.30 & 0.10  & 5.00  & 0.00 & 0.00   & -1.00  & 0.00   & 49.69 & 15.55          & 22.56  \\
body 1  & 0.37 & 0.05  & 5.96  & 0.20 & 0.75   & 0.67   & 0.00   & 49.69 & 15.55          & 22.56  \\
body 2  & 0.37 & 0.05  & 5.96  & 0.20 & -0.75  & 0.67   & 0.00   & 49.69 & 15.55          & 22.56  \\
body 3  & 1.44 & 0.06  & 4.77  & 1.00 & 0.72   & 0.41   & -0.56  & 49.69 & 15.55          & 22.56  \\
body 4  & 1.44 & 0.06  & 4.77  & 1.00 & -0.72  & 0.41   & -0.56  & 49.69 & 15.55          & 22.56  \\
body 5  & 0.30 & 0.10  & 5.00  & 1.00 & 0.00   & -1.00  & 0.00   & 49.69 & 15.55          & 22.56  \\
body 6  & 0.30 & 0.10  & 5.00  & 1.00 & 0.00   & -1.00  & 0.00   & 49.69 & 15.55          & 22.56  \\
body 7  & 0.46 & 0.05  & 3.46  & 0.80 & 0.88   & -0.34  & 0.00   & 49.69 & 15.55          & 22.56  \\
body 8  & 0.46 & 0.05  & 3.46  & 0.80 & -0.88  & -0.34  & 0.00   & 49.69 & 15.55          & 22.56  \\
body 9  & 1.10 & 0.05  & 4.75  & 1.00 & 0.36   & -0.41  & -0.85  & 49.69 & 15.55          & 22.56  \\
body 10 & 1.10 & 0.05  & 4.75  & 1.00 & -0.36  & -0.41  & -0.85  & 49.69 & 15.55          & 22.56  \\
\midrule
\textbf{Delta}   & 4.55 & -7.37 & -4.01 & 0.00 & 0.00   & -27.89 & -16.08 & -0.62 & 3.53           & 11.33\\
\midrule
        &             &             &              &               &               &               &              &             & \textbf{Actual Change:} & \color[HTML]{FF0000} 3.66\% \\
\midrule
\multicolumn{11}{c}{\textbf{Evolved} (fixed legs)}                                                                                                                          \\
\midrule
\textbf{avg}    & 0.67 & 0.07  & 4.98  & 0.73 & 0.01   & -0.27  & -0.30  & 50.08 & 12.44          & 17.12  \\
body 0  & 0.32 & 0.08  & 4.70  & 0.00 & 0.00   & -1.00  & 0.00   & 50.08 & 12.44          & 17.12  \\
body 1  & 0.40 & 0.06  & 5.00  & 0.20 & 0.71   & 0.71   & 0.00   & 50.08 & 12.44          & 17.12  \\
body 2  & 0.40 & 0.06  & 5.00  & 0.20 & -0.71  & 0.71   & 0.00   & 50.08 & 12.44          & 17.12  \\
body 3  & 1.20 & 0.06  & 5.00  & 1.00 & 0.41   & 0.41   & -0.82  & 50.08 & 12.44          & 17.12  \\
body 4  & 1.20 & 0.06  & 5.00  & 1.00 & -0.41  & 0.41   & -0.82  & 50.08 & 12.44          & 17.12  \\
body 5  & 0.25 & 0.12  & 4.42  & 1.00 & 0.14   & -0.99  & 0.00   & 50.08 & 12.44          & 17.12  \\
body 6  & 0.35 & 0.10  & 5.64  & 1.00 & -0.02  & -1.00  & 0.00   & 50.08 & 12.44          & 17.12  \\
body 7  & 0.40 & 0.06  & 5.00  & 0.80 & 0.71   & -0.71  & 0.00   & 50.08 & 12.44          & 17.12  \\
body 8  & 0.40 & 0.06  & 5.00  & 0.80 & -0.71  & -0.71  & 0.00   & 50.08 & 12.44          & 17.12  \\
body 9  & 1.20 & 0.06  & 5.00  & 1.00 & 0.41   & -0.41  & -0.82  & 50.08 & 12.44          & 17.12  \\
body 10 & 1.20 & 0.06  & 5.00  & 1.00 & -0.41  & -0.41  & -0.82  & 50.08 & 12.44          & 17.12  \\
\midrule
\textbf{Delta}   & 0.41 & -0.24 & -0.44 & 0.00 & 100.00 & -0.35  & 0.00   & 0.17  & -20.55         & -16.83\\
\midrule
        &             &             &              &               &               &               &              &             & \textbf{Actual Change:} & \color[HTML]{FF0000} 6.22\% \\
\bottomrule
\end{tabular}
\caption{Detailed comparison between baseline and evolved agent of Fig.  \ref{fig:expD}.}\label{table:expD}
\end{table*}

%%%%%%%%%%%%%%%%%%%%%%%%%%%%%%%%%%%%%%%%%%%%%%%%%%%%%%%%
%%%%%%%%%%%%%%%%%%%%%%%%%%%%%%%%%%%%%%%%%%%%%%%%%%%%%%%%
%%%%%%%%%%%%%%%%%%%%%%%%%%%%%%%%%%%%%%%%%%%%%%%%%%%%%%%%
%%%%%%%%%%%%%%%%%%%%%%%%%%%%%%%%%%%%%%%%%%%%%%%%%%%%%%%%
%%%%%%%%%%%%%%%%%%%%%%%%%%%%%%%%%%%%%%%%%%%%%%%%%%%%%%%%
%%%%%%%%%%%%%%%%%%%%%%%%%%%%%%%%%%%%%%%%%%%%%%%%%%%%%%%%
%%%%%%%%%%%%%%%%%%%%%%%%%%%%%%%%%%%%%%%%%%%%%%%%%%%%%%%%

\begin{table*}[!htb]
%\scriptsize
\begin{tabular}{lllllllllll}
\toprule
\multicolumn{11}{c}{\textbf{Baseline} (Agent in Fig.  \ref{fig:expA} (a))}                                                                                                                                  \\
\midrule
& \textbf{Length}  & \textbf{Radius}      & \textbf{Density}     & \textbf{Initial Pos}  & \textbf{Initial Dir} $x$ & \textbf{Initial Dir} $y$ & \textbf{Initial Dir} $z$ & \textbf{Stiffness}    & \textbf{Damping}     & \textbf{Max Effort}              \\
\midrule
\textbf{avg}    & 0.40       & 0.07       & 5.00        & 0.75          & 0.00          & -0.33         & -0.24      & 5.00       & 2.00          & 5.00                              \\
body 0  & 0.40       & 0.10       & 5.00        & 0.00          & 0.00          & -1.00         & 0.00       & 5.00       & 2.00          & 5.00                              \\
body 1  & 0.40       & 0.10       & 5.00        & 1.00          & 0.00          & -1.00         & 0.00       & 5.00       & 2.00          & 5.00                              \\
body 2  & 0.40       & 0.06       & 5.00        & 0.20          & -1.00         & 0.00          & 0.00       & 5.00       & 2.00          & 5.00                              \\
body 3  & 0.40       & 0.06       & 5.00        & 0.20          & 1.00          & 0.00          & 0.00       & 5.00       & 2.00          & 5.00                              \\
body 4  & 0.40       & 0.06       & 5.00        & 1.00          & -0.71         & 0.00          & -0.71      & 5.00       & 2.00          & 5.00                              \\
body 5  & 0.40       & 0.06       & 5.00        & 1.00          & 0.71          & 0.00          & -0.71      & 5.00       & 2.00          & 5.00                              \\
body 6  & 0.40       & 0.10       & 5.00        & 1.00          & 0.00          & -1.00         & 0.00       & 5.00       & 2.00          & 5.00                              \\
body 7  & 0.40       & 0.06       & 5.00        & 0.80          & 1.00          & 0.00          & 0.00       & 5.00       & 2.00          & 5.00                              \\
body 8  & 0.40       & 0.06       & 5.00        & 0.80          & -1.00         & 0.00          & 0.00       & 5.00       & 2.00          & 5.00                              \\
body 9  & 0.40       & 0.06       & 5.00        & 1.00          & 0.71          & 0.00          & -0.71      & 5.00       & 2.00          & 5.00                              \\
body 10 & 0.40       & 0.06       & 5.00        & 1.00          & -0.71         & 0.00          & -0.71      & 5.00       & 2.00          & 5.00                              \\
body 11 & 0.40       & 0.10       & 5.00        & 1.00          & 0.00          & -1.00         & 0.00       & 5.00       & 2.00          & 5.00                              \\
\midrule
\multicolumn{11}{c}{\textbf{Evolved} $\pm10\%$ (Agent in Fig.  \ref{fig:expA} (b))}                                                                                                                          \\
\midrule
\textbf{avg}     & 0.41      & 0.07       & 4.90        & 0.75          & 0.01          & -0.31         & -0.23      & 5.27       & 1.90          & 4.85                              \\
body 0  & 0.42      & 0.10       & 5.35        & 0.00          & 0.00          & -1.00         & 0.00       & 5.27       & 1.90          & 4.85                              \\
body 1  & 0.38      & 0.11       & 4.85        & 1.00          & -0.16         & -0.99         & 0.00       & 5.27       & 1.90          & 4.85                              \\
body 2  & 0.41      & 0.06       & 5.16        & 0.20          & -1.00         & -0.04         & 0.00       & 5.27       & 1.90          & 4.85                              \\
body 3  & 0.41      & 0.06       & 5.16        & 0.20          & 1.00          & -0.04         & 0.00       & 5.27       & 1.90          & 4.85                              \\
body 4  & 0.42      & 0.06       & 4.99        & 1.00          & -0.72         & 0.00          & -0.70      & 5.27       & 1.90          & 4.85                              \\
body 5  & 0.42      & 0.06       & 4.99        & 1.00          & 0.72          & 0.00          & -0.70      & 5.27       & 1.90          & 4.85                              \\
body 6  & 0.43      & 0.11       & 4.51        & 1.00          & 0.12          & -0.99         & 0.00       & 5.27       & 1.90          & 4.85                              \\
body 7  & 0.41      & 0.07       & 4.32        & 0.80          & 0.98          & 0.18          & 0.00       & 5.27       & 1.90          & 4.85                              \\
body 8  & 0.41      & 0.07       & 4.32        & 0.80          & -0.98         & 0.18          & 0.00       & 5.27       & 1.90          & 4.85                              \\
body 9  & 0.41      & 0.06       & 5.19        & 1.00          & 0.81          & 0.00          & -0.70      & 5.27       & 1.90          & 4.85                              \\
body 10 & 0.41      & 0.06       & 5.19        & 1.00          & -0.81         & 0.00          & -0.70      & 5.27       & 1.90          & 4.85                              \\
body 11 & 0.38      & 0.09       & 4.78        & 1.00          & 0.11          & -0.99         & 0.00       & 5.27       & 1.90          & 4.85                              \\
\midrule
\textbf{Delta}   & 2.17 & 1.78 & -1.98 & 0             & 100.00           & -8.06  & -1.14 & 5.09 & -5.25   & -3.11 \\
\midrule
        &             &             &              &               &               &               &              &             & \textbf{Actual Change:} & \color[HTML]{FF0000} 8.94\% \\
\midrule
\multicolumn{11}{c}{\textbf{Evolved} $\pm20\%$ (Agent in Fig.  \ref{fig:expA} (c))}                                                                                                                          \\
\midrule
\textbf{avg}     & 0.43      & 0.08       & 4.91        & 0.75          & -0.03         & -0.32         & -0.17      & 5.93       & 2.24          & 5.97                              \\
body 0  & 0.36      & 0.12       & 5.77        & 0.00          & 0.00          & -1.00         & 0.00       & 5.93       & 2.24          & 5.97                              \\
body 1  & 0.46      & 0.11       & 5.45        & 1.00          & 0.04          & -1.00         & 0.00       & 5.93       & 2.24          & 5.97                              \\
body 2  & 0.41      & 0.05       & 5.29        & 0.20          & -1.00         & 0.10          & 0.00       & 5.93       & 2.24          & 5.97                              \\
body 3  & 0.41      & 0.05       & 5.29        & 0.20          & 1.00          & 0.10          & 0.00       & 5.93       & 2.24          & 5.97                              \\
body 4  & 0.42      & 0.07       & 4.76        & 1.00          & -0.83         & 0.00          & -0.56      & 5.93       & 2.24          & 5.97                              \\
body 5  & 0.42      & 0.07       & 4.76        & 1.00          & 0.83          & 0.00          & -0.56      & 5.93       & 2.24          & 5.97                              \\
body 6  & 0.42      & 0.08       & 4.50        & 1.00          & -0.14         & -1.00         & 0.00       & 5.93       & 2.24          & 5.97                              \\
body 7  & 0.42      & 0.07       & 3.51        & 0.80          & 1.00          & -0.04         & 0.00       & 5.93       & 2.24          & 5.97                              \\
body 8  & 0.42      & 0.07       & 3.51        & 0.80          & -1.00         & -0.04         & 0.00       & 5.93       & 2.24          & 5.97                              \\
body 9  & 0.53      & 0.07       & 5.55        & 1.00          & 0.64          & 0.00          & -0.49      & 5.93       & 2.24          & 5.97                              \\
body 10 & 0.53      & 0.07       & 5.55        & 1.00          & -0.64         & 0.00          & -0.49      & 5.93       & 2.24          & 5.97                              \\
body 11 & 0.35      & 0.08       & 5.00        & 1.00          & -0.27         & -1.00         & 0.00       & 5.93       & 2.24          & 5.97                              \\
\midrule
\textbf{Delta}   & 6.45  & 4.43  & -1.79  & 0.00             & 100.00           & -3.08    & -35.19   & 15.74 & 10.85    & 16.20                        \\
\midrule
&            &             &             &               &               &               &              &            & \textbf{Actual Change} & {\color[HTML]{FF0000} 11.36\%}\\
\bottomrule
\end{tabular}
\caption{Detailed comparison between baseline (Fig.  \ref{fig:expA} (a)) and evolved agents (Fig.  \ref{fig:expA} (b) and Fig.  \ref{fig:expA} (c)).}\label{table:expA}
\end{table*}

\begin{table*}[!htb]
\scriptsize
\begin{tabular}{lllllllllll}
\toprule
\multicolumn{11}{c}{\textbf{Baseline}}                                                                                                                                  \\
\midrule
& \textbf{Length}  & \textbf{Radius}      & \textbf{Density}     & \textbf{Initial Pos}  & \textbf{Initial Dir} $x$ & \textbf{Initial Dir} $y$ & \textbf{Initial Dir} $z$ & \textbf{Stiffness}    & \textbf{Damping}     & \textbf{Max Effort}              \\
\midrule
\textbf{avg}   & 0.34 & 0.09  & 5.17  & 0.88 & -0.08  & -0.03   & 0.02  & 5.00 & 2.00           & 10.00  \\
body 0 & 0.33 & 0.12  & 5.85  & 1.00 & 0.00   & -1.00   & 0.00  & 5.00 & 2.00           & 10.00  \\
body 1 & 0.32 & 0.17  & 6.68  & 1.00 & 0.00   & -0.99   & 0.17  & 5.00 & 2.00           & 10.00  \\
body 2 & 0.38 & 0.08  & 3.10  & 0.50 & 1.00   & 0.09    & 0.00  & 5.00 & 2.00           & 10.00  \\
body 3 & 0.31 & 0.08  & 5.74  & 1.00 & 0.94   & 0.34    & 0.00  & 5.00 & 2.00           & 10.00  \\
body 4 & 0.38 & 0.08  & 6.02  & 1.00 & 0.22   & 0.98    & 0.00  & 5.00 & 2.00           & 10.00  \\
body 5 & 0.33 & 0.08  & 3.27  & 0.50 & -1.00  & 0.00    & 0.00  & 5.00 & 2.00           & 10.00  \\
body 6 & 0.40 & 0.08  & 3.79  & 1.00 & -0.96  & -0.27   & 0.00  & 5.00 & 2.00           & 10.00  \\
body 7 & 0.30 & 0.08  & 6.87  & 1.00 & -0.82  & 0.58    & 0.00  & 5.00 & 2.00           & 10.00  \\
\midrule
\multicolumn{11}{c}{\textbf{Evolved} $\pm20\%$}                                                                                                                          \\
\midrule
\textbf{avg}    & 0.36 & 0.09  & 5.11  & 0.88 & -0.07  & -0.01   & 0.03  & 5.12 & 2.09           & 10.45  \\
body 0 & 0.36 & 0.11  & 5.80  & 1.00 & 0.00   & -1.00   & 0.00  & 5.12 & 2.09           & 10.45  \\
body 1 & 0.33 & 0.17  & 6.15  & 1.00 & 0.00   & -0.98   & 0.20  & 5.12 & 2.09           & 10.45  \\
body 2 & 0.40 & 0.07  & 3.39  & 0.50 & 0.99   & 0.11    & 0.00  & 5.12 & 2.09           & 10.45  \\
body 3 & 0.34 & 0.08  & 5.64  & 1.00 & 0.94   & 0.45    & 0.00  & 5.12 & 2.09           & 10.45  \\
body 4 & 0.39 & 0.08  & 5.84  & 1.00 & 0.36   & 0.95    & 0.00  & 5.12 & 2.09           & 10.45  \\
body 5 & 0.35 & 0.08  & 3.42  & 0.50 & -1.00  & 0.00    & 0.00  & 5.12 & 2.09           & 10.45  \\
body 6 & 0.42 & 0.07  & 3.47  & 1.00 & -0.95  & -0.30   & 0.00  & 5.12 & 2.09           & 10.45  \\
body 7 & 0.29 & 0.08  & 7.18  & 1.00 & -0.88  & 0.66    & 0.00  & 5.12 & 2.09           & 10.45  \\
\midrule
\textbf{Delta}   & 4.41 & -0.91 & -1.08 & 0.00 & -16.02 & -183.08 & 17.40 & 2.40 & 4.20           & 4.32 \\
\midrule
        &             &             &              &               &               &               &              &             & \textbf{Actual Change:} & \color[HTML]{FF0000} 16.84\% \\
\bottomrule
\end{tabular}
\caption{Detailed comparison between baseline and evolved agent of Fig.  \ref{fig:expBa}.}\label{table:expBa}
\end{table*}

\begin{table*}[!htb]
\scriptsize
\begin{tabular}{lllllllllll}
\toprule
\multicolumn{11}{c}{\textbf{Baseline}}                                                                                                                                  \\
\midrule
& \textbf{Length}  & \textbf{Radius}      & \textbf{Density}     & \textbf{Initial Pos}  & \textbf{Initial Dir} $x$ & \textbf{Initial Dir} $y$ & \textbf{Initial Dir} $z$ & \textbf{Stiffness}    & \textbf{Damping}     & \textbf{Max Effort}              \\
\midrule
\textbf{avg}   & 0.35  & 0.07 & 5.00  & 0.83 & 0.00   & -0.23 & -0.14 & 5.00  & 2.00           & 5.00  \\
body 0  & 0.30  & 0.10 & 5.00  & 0.00 & 0.00   & -1.00 & 0.00  & 5.00  & 2.00           & 5.00  \\
body 1  & 0.40  & 0.06 & 5.00  & 0.80 & 1.00   & 0.00  & 0.00  & 5.00  & 2.00           & 5.00  \\
body 2  & 0.40  & 0.06 & 5.00  & 0.80 & -1.00  & 0.00  & 0.00  & 5.00  & 2.00           & 5.00  \\
body 3  & 0.30  & 0.06 & 5.00  & 1.00 & 0.71   & 0.00  & 0.71  & 5.00  & 2.00           & 5.00  \\
body 4  & 0.30  & 0.06 & 5.00  & 1.00 & -0.71  & 0.00  & 0.71  & 5.00  & 2.00           & 5.00  \\
body 5  & 0.40  & 0.06 & 5.00  & 1.00 & 0.45   & 0.00  & -0.89 & 5.00  & 2.00           & 5.00  \\
body 6  & 0.40  & 0.06 & 5.00  & 1.00 & -0.45  & 0.00  & -0.89 & 5.00  & 2.00           & 5.00  \\
body 7  & 0.30  & 0.10 & 5.00  & 1.00 & 0.00   & -1.00 & 0.00  & 5.00  & 2.00           & 5.00  \\
body 8  & 0.30  & 0.10 & 5.00  & 1.00 & 0.00   & -1.00 & 0.00  & 5.00  & 2.00           & 5.00  \\
body 9  & 0.40  & 0.06 & 5.00  & 0.60 & 1.00   & 0.00  & 0.00  & 5.00  & 2.00           & 5.00  \\
body 10 & 0.40  & 0.06 & 5.00  & 0.60 & -1.00  & 0.00  & 0.00  & 5.00  & 2.00           & 5.00  \\
body 11 & 0.30  & 0.06 & 5.00  & 1.00 & 0.71   & 0.00  & -0.71 & 5.00  & 2.00           & 5.00  \\
body 12 & 0.30  & 0.06 & 5.00  & 1.00 & -0.71  & 0.00  & -0.71 & 5.00  & 2.00           & 5.00  \\
\midrule
\multicolumn{11}{c}{\textbf{Evolved} $\pm20\%$}                                                                                                                          \\
\midrule
\textbf{avg}    & 0.47  & 0.07 & 4.92  & 0.83 & 0.02   & -0.30 & -0.14 & 4.84  & 2.19           & 5.47  \\
body 0  & 0.56  & 0.10 & 4.34  & 0.00 & 0.00   & -1.00 & 0.00  & 4.84  & 2.19           & 5.47  \\
body 1  & 0.34  & 0.06 & 4.64  & 0.80 & 0.91   & -0.05 & 0.00  & 4.84  & 2.19           & 5.47  \\
body 2  & 0.47  & 0.06 & 3.01  & 0.80 & -0.91  & -0.05 & 0.00  & 4.84  & 2.19           & 5.47  \\
body 3  & 0.47  & 0.06 & 5.67  & 1.00 & 0.77   & 0.00  & 0.64  & 4.84  & 2.19           & 5.47  \\
body 4  & 0.47  & 0.06 & 3.19  & 1.00 & -0.77  & 0.00  & 0.71  & 4.84  & 2.19           & 5.47  \\
body 5  & 0.59  & 0.06 & 6.88  & 1.00 & 0.33   & 0.00  & -0.94 & 4.84  & 2.19           & 5.47  \\
body 6  & 0.59  & 0.06 & 6.88  & 1.00 & -0.33  & 0.00  & -0.98 & 4.84  & 2.19           & 5.47  \\
body 7  & 0.42  & 0.10 & 2.59  & 1.00 & 0.00   & -0.99 & -0.08 & 4.84  & 2.19           & 5.47  \\
body 8  & 0.31  & 0.10 & 4.54  & 1.00 & 0.34   & -0.94 & 0.00  & 4.84  & 2.19           & 5.47  \\
body 9  & 0.52  & 0.06 & 4.18  & 0.60 & 1.00   & -0.46 & 0.00  & 4.84  & 2.19           & 5.47  \\
body 10 & 0.52  & 0.06 & 5.98  & 0.60 & -1.00  & -0.46 & 0.00  & 4.84  & 2.19           & 5.47  \\
body 11 & 0.46  & 0.06 & 6.06  & 1.00 & 0.78   & 0.00  & -0.53 & 4.84  & 2.19           & 5.47  \\
body 12 & 0.37  & 0.06 & 6.06  & 1.00 & -0.85  & 0.00  & -0.62 & 4.84  & 2.19           & 5.47  \\
\midrule
\textbf{Delta}   & 26.10 & 0.00 & -1.53 & 0.00 & 100.00 & 24.24 & 1.26  & -3.39 & 8.48           & 8.61 \\
\midrule
        &             &             &              &               &               &               &              &             & \textbf{Actual Change:} & \color[HTML]{FF0000} 16.38\% \\
\bottomrule
\end{tabular}
\caption{Detailed comparison between baseline and evolved agent of Fig.  \ref{fig:expBb}.}\label{table:expBb}
\end{table*}

\begin{table*}[!htb]
\scriptsize
\begin{tabular}{lllllllllll}
\toprule
\multicolumn{11}{c}{\textbf{Baseline}}                                                                                                                                  \\
\midrule
& \textbf{Length}  & \textbf{Radius}      & \textbf{Density}     & \textbf{Initial Pos}  & \textbf{Initial Dir} $x$ & \textbf{Initial Dir} $y$ & \textbf{Initial Dir} $z$ & \textbf{Stiffness}    & \textbf{Damping}     & \textbf{Max Effort}              \\
\midrule
\textbf{avg}   & 0.30  & 0.07  & 5.00 & 0.82  & 0.00   & -0.33 & -0.24 & 50.00 & 15.00 & 500.00 \\
body 0  & 0.30  & 0.10  & 5.00 & 0.00  & 0.00   & -1.00 & 0.00  & 50.00 & 15.00 & 500.00 \\
body 1  & 0.40  & 0.06  & 5.00 & 0.80  & 1.00   & 0.00  & 0.00  & 50.00 & 15.00 & 500.00 \\
body 2  & 0.20  & 0.06  & 5.00 & 1.00  & 0.71   & 0.00  & -0.71 & 50.00 & 15.00 & 500.00 \\
body 3  & 0.30  & 0.10  & 5.00 & 1.00  & 0.00   & -1.00 & 0.00  & 50.00 & 15.00 & 500.00 \\
body 4  & 0.40  & 0.06  & 5.00 & 0.60  & -1.00  & 0.00  & 0.00  & 50.00 & 15.00 & 500.00 \\
body 5  & 0.20  & 0.06  & 5.00 & 1.00  & -0.71  & 0.00  & -0.71 & 50.00 & 15.00 & 500.00 \\
body 6  & 0.30  & 0.10  & 5.00 & 1.00  & 0.00   & -1.00 & 0.00  & 50.00 & 15.00 & 500.00 \\
body 7  & 0.40  & 0.06  & 5.00 & 0.60  & 1.00   & 0.00  & 0.00  & 50.00 & 15.00 & 500.00 \\
body 8  & 0.20  & 0.06  & 5.00 & 1.00  & 0.71   & 0.00  & -0.71 & 50.00 & 15.00 & 500.00 \\
body 9  & 0.30  & 0.10  & 5.00 & 1.00  & 0.00   & -1.00 & 0.00  & 50.00 & 15.00 & 500.00 \\
body 10 & 0.40  & 0.06  & 5.00 & 0.60  & -1.00  & 0.00  & 0.00  & 50.00 & 15.00 & 500.00 \\
body 11 & 0.20  & 0.06  & 5.00 & 1.00  & -0.71  & 0.00  & -0.71 & 50.00 & 15.00 & 500.00 \\
body 12 & 0.30  & 0.10  & 5.00 & 1.00  & 0.00   & -1.00 & 0.00  & 50.00 & 15.00 & 500.00 \\
body 13 & 0.40  & 0.06  & 5.00 & 0.60  & 1.00   & 0.00  & 0.00  & 50.00 & 15.00 & 500.00 \\
body 14 & 0.20  & 0.06  & 5.00 & 1.00  & 0.71   & 0.00  & -0.71 & 50.00 & 15.00 & 500.00 \\
body 15 & 0.30  & 0.10  & 5.00 & 1.00  & 0.00   & -1.00 & 0.00  & 50.00 & 15.00 & 500.00 \\
body 16 & 0.40  & 0.06  & 5.00 & 0.60  & -1.00  & 0.00  & 0.00  & 50.00 & 15.00 & 500.00 \\
body 17 & 0.20  & 0.06  & 5.00 & 1.00  & -0.71  & 0.00  & -0.71 & 50.00 & 15.00 & 500.00 \\
body 18 & 0.30  & 0.10  & 5.00 & 1.00  & 0.00   & -1.00 & 0.00  & 50.00 & 15.00 & 500.00 \\
body 19 & 0.40  & 0.06  & 5.00 & 0.60  & 1.00   & 0.00  & 0.00  & 50.00 & 15.00 & 500.00 \\
body 20 & 0.20  & 0.06  & 5.00 & 1.00  & 0.71   & 0.00  & -0.71 & 50.00 & 15.00 & 500.00  \\
\midrule
\multicolumn{11}{c}{\textbf{Evolved} $\pm20\%$}                                                                                                                          \\
\midrule
\textbf{avg}    & 0.30  & 0.07  & 5.04 & 0.81  & 0.00   & -0.33 & -0.25 & 50.39 & 14.07 & 526.56 \\
body 0  & 0.31  & 0.10  & 5.17 & 0.00  & 0.00   & -1.01 & 0.00  & 50.39 & 14.07 & 526.56 \\
body 1  & 0.37  & 0.06  & 4.79 & 0.80  & 0.99   & 0.09  & 0.00  & 50.39 & 14.07 & 526.56 \\
body 2  & 0.19  & 0.06  & 5.12 & 1.00  & 0.69   & 0.00  & -0.78 & 50.39 & 14.07 & 526.56 \\
body 3  & 0.28  & 0.10  & 5.16 & 0.98  & -0.04  & -1.09 & 0.00  & 50.39 & 14.07 & 526.56 \\
body 4  & 0.46  & 0.05  & 5.18 & 0.54  & -0.98  & -0.05 & 0.00  & 50.39 & 14.07 & 526.56 \\
body 5  & 0.20  & 0.07  & 5.07 & 1.00  & -0.62  & 0.00  & -0.79 & 50.39 & 14.07 & 526.56 \\
body 6  & 0.28  & 0.09  & 4.52 & 0.96  & -0.01  & -1.00 & 0.00  & 50.39 & 14.07 & 526.56 \\
body 7  & 0.41  & 0.06  & 5.16 & 0.60  & 1.00   & 0.12  & 0.00  & 50.39 & 14.07 & 526.56 \\
body 8  & 0.19  & 0.07  & 5.49 & 1.00  & 0.75   & 0.00  & -0.77 & 50.39 & 14.07 & 526.56 \\
body 9  & 0.29  & 0.09  & 5.14 & 1.00  & -0.02  & -1.00 & 0.00  & 50.39 & 14.07 & 526.56 \\
body 10 & 0.38  & 0.07  & 5.19 & 0.60  & -1.11  & -0.13 & 0.00  & 50.39 & 14.07 & 526.56 \\
body 11 & 0.22  & 0.06  & 5.32 & 1.00  & -0.74  & 0.00  & -0.67 & 50.39 & 14.07 & 526.56 \\
body 12 & 0.29  & 0.11  & 4.57 & 1.00  & 0.11   & -1.03 & 0.00  & 50.39 & 14.07 & 526.56 \\
body 13 & 0.39  & 0.06  & 4.79 & 0.56  & 1.00   & 0.08  & 0.00  & 50.39 & 14.07 & 526.56 \\
body 14 & 0.21  & 0.05  & 5.49 & 1.00  & 0.65   & 0.00  & -0.76 & 50.39 & 14.07 & 526.56 \\
body 15 & 0.30  & 0.10  & 4.79 & 1.00  & 0.05   & -0.99 & 0.00  & 50.39 & 14.07 & 526.56 \\
body 16 & 0.43  & 0.06  & 4.95 & 0.60  & -1.00  & 0.02  & 0.00  & 50.39 & 14.07 & 526.56 \\
body 17 & 0.19  & 0.05  & 4.75 & 1.00  & -0.81  & 0.00  & -0.67 & 50.39 & 14.07 & 526.56 \\
body 18 & 0.30  & 0.11  & 5.34 & 1.01  & 0.02   & -1.04 & 0.00  & 50.39 & 14.07 & 526.56 \\
body 19 & 0.43  & 0.06  & 4.69 & 0.60  & 1.00   & -0.04 & 0.00  & 50.39 & 14.07 & 526.56 \\
body 20 & 0.20  & 0.06  & 4.90 & 1.03  & 0.83   & 0.00  & -0.65 & 50.39 & 14.07 & 526.56  \\
\midrule
\textbf{Delta}   & -0.23 & -1.45 & 0.73 & -1.08 & 100.00 & 0.05  & 4.47  & 0.78  & -6.57 & 5.04 \\
\midrule
        &             &             &              &               &               &               &              &             & \textbf{Actual Change:} & \color[HTML]{FF0000} 10.17\% \\
\bottomrule
\end{tabular}
\caption{Detailed comparison between baseline and evolved agent of Fig.  \ref{fig:expBc}.}\label{table:expBc}
\end{table*}
